# Supplementary material for: Rotational and translational dynamics in dense fluids of patchy particles
Source: arXiv:2002.01902 ancillary file (2020-02-05)
Supplement: Supplementary file 1 [file SI.pdf]

# Rotational and translational dynamics in dense fluids of patchy particles: Supplemental Information

Susana Marín-Aguilar, Henricus H. Wensink, Giuseppe Foffi,* and Frank Smallenburg†
*Université Paris-Saclay, CNRS, Laboratoire de Physique des Solides, 91405, Orsay, France*

## ROTATIONAL DYNAMICS

The behavior of the rotational correlation is highly dependent on the size of the patches and the temperature. As discussed in the main text, the rotational correlation functions hint at the presence of free spinners, due to the presence of a local minimum in the correlation function at short time scales. To support his, we show in Fig. S1 the rotational correlation of a system of hard spheres. This was measured in the same way as in the patchy systems, by fixing a vector in each of the particles and following its motion. There is a fast decay of the correlation and then a sudden increase corresponding to the rotation of the free spinners back to their original configuration. For long time scales, the average over many spinners with different rotation periods and angles between the spinning axis and the chosen "patch" vector causes the correlation function to level off to a plateau. Note that, since in these systems the spinning axis never changes, the orientations never fully decorrelate.

In the same figure we show one of the patchy systems where we found the local minimum in the correlation function. The time at the minimum indeed matches between the two cases. This confirms our conclusion that this minimum results from the presence of free spinners in the system.

Furthermore, in Fig. S2 we show the rotational correlation functions for selected angles of the 6-patch case to illustrate the dependence of the size of the patches and the temperature. For smaller patch angles $\theta$, the effect of the free-spinners is found in a wider range of temperatures, as can be seen in Fig. S2a, where after the initial decay in the correlation function we observe an oscillatory behavior. The short plateau related to the bonding with the particles in the local cage is present at lower temperatures and larger patch-sizes as it is shown in S2b, c, and d.

In Fig. S3 we show the rotational correlation of the 12-patch case where the same behavior is found.

* Electronic address: giuseppe.foffi@u-psud.fr
† Electronic address: frank.smallenburg@u-psud.fr

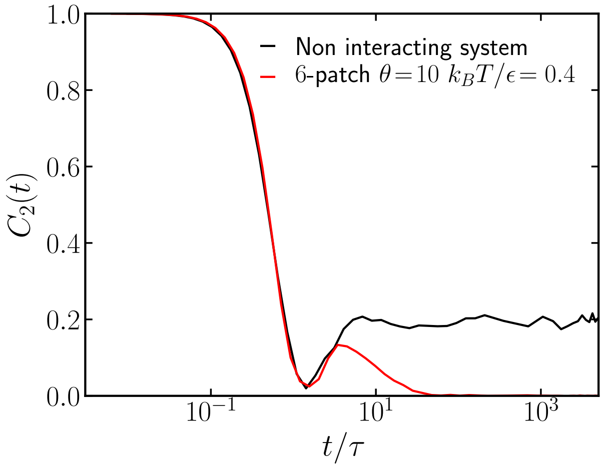


FIG. S1: Rotational correlation functions of a system of non interacting particles and the 6-patch case for an opening angle of 10° and $k_BT/\epsilon = 0.4$. In both cases, the packing fraction is fixed at $\eta = 0.58$.

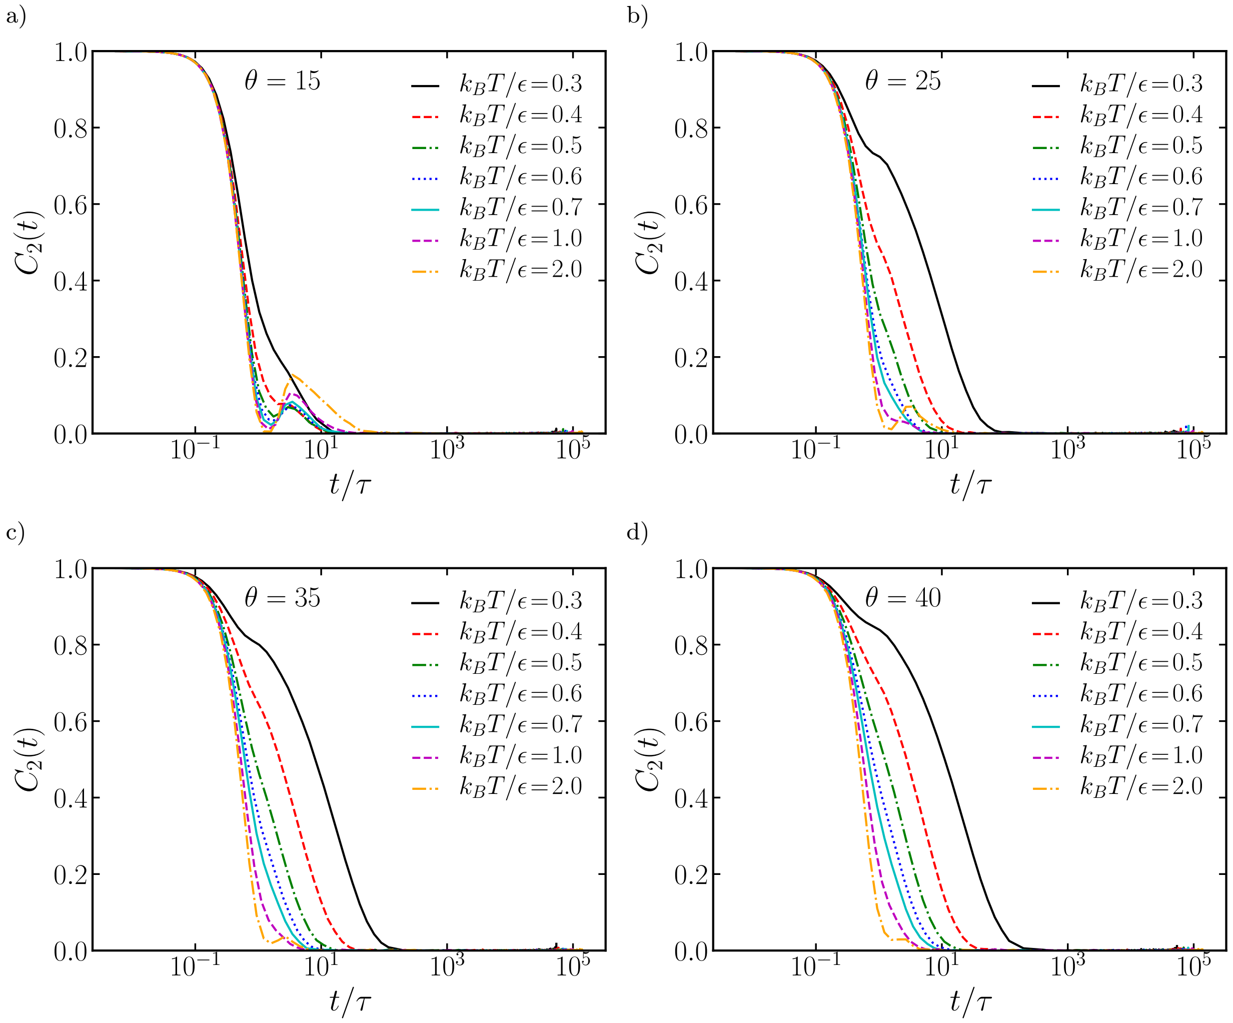


FIG. S2: Rotational correlation functions of the 6-patch case for an opening angle of a) 15°, b) 25°, c) 35° and d) 40°. In all cases, the packing fraction is fixed at $\eta = 0.58$.

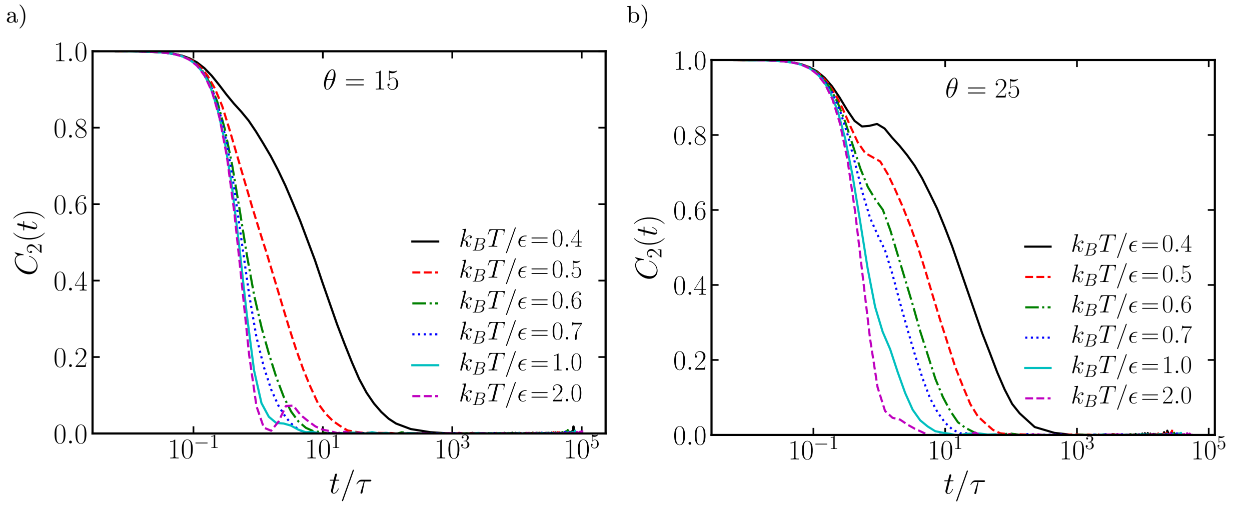


FIG. S3: Rotational correlation functions of the 12-patch case for an opening angle of a) 15° and b) 25°. In all cases, the packing fraction is fixed at $\eta = 0.58$.
